# Supplementary material for: Harnessing the Power of LLMs: Evaluating Human-AI Text Co-Creation through the Lens of News Headline Generation
Source: arXiv:2310.10706 source file (2023-10-18)
Supplement: Supplementary file 1 [file 20_news_dataset.tex]

Criteria:
Not about US Politics / Political issues (which can be under US, Politics, World, even others)
Not too short >300 words (300~1000 words is common on Yahoo! News, usually ~500 words)

Example
U.N. Security Council extends Haiti political mission, declines to expand it amid gang crisis
[title]

The United Nations Security Council voted unanimously on Friday to extend the mandate of the U.N. Integrated Office in Haiti, which would otherwise have expired Friday, for one year, but did not provide additional security assistance to the country as it faces its gravest spate of violence in years.

The council adopted the resolution, drafted by the United States and Mexico, after extensive consultation between the United States and China. Beijing had been pushing for stronger language that would impose a ban on arms and munitions sales to Haitian gangs.

“The mandate reflects the key challenges facing Haiti, including the need to address illegal arms trafficking and illicit financial flows, and that the Security Council is ready to consider taking measures, as appropriate, to address these challenges,” Jeffrey DeLaurentis, a U.S. diplomat, told the council after the vote.

“We must also note it is long past time for Haiti’s stakeholders to set aside their differences,” he added, “and to reach agreement on a political framework that will allow Haiti to hold presidential and legislative elections when conditions permit.”

A representative of Mexico, Juan Ramón de la Fuente Ramirez, told the Security Council that the resolution “calls for a cessation of violence.”

The U.N. political mission in Haiti was established in 2019 to promote stability in Port-au-Prince.

But the ongoing security crisis in Haiti, which has been devastated by gang violence and political paralysis since the assassination of its president last year, led some to call for a more robust security package to accompany the renewal.

China’s diplomat, Zhang Jun, said that more could have been done, but that several of its proposals had been incorporated into the U.S.-Mexico draft.

“This resolution raises clear warnings to the gangs that the Security Council is closely following their actions,” said Zhang. “For individuals who are gang members or supporters of gang activities, the Security Council will soon impose sanctions in accordance to the relevant provisions of the U.N. charter to seriously hold them accountable.”

“Haiti has been one of the most complicated and intractable challenges on the council’s agenda,” China’s diplomat said, describing the current situation in Haiti as a “more severe crisis” than the country has faced in 30 years.

Hawaiian waters may get too hot for humpback whales due to climate change
[title]

The warm, shallow waters near Hawaii are a renowned breeding ground for humpback whales. An estimated two-thirds of North Pacific humpback whales are born there, and the massive creatures — adult males can be up to 52 feet long and can weigh 45 tons — figure in the mythology of native Hawaiians. For the locals who make their living giving tours to whale-watching visitors, they are also an important part of the state’s economy.

But that may all be upended in the decades to come, due to climate change — and the more greenhouse gases that are emitted this century, the fewer whales there will be in Hawaii, according to a new study.

Humpback whales give birth in waters that range from about 70°F to 82°F, but at their current pace of warming, two-thirds of the waters near Hawaii will surpass 82°F by the end of this century, the study found.

The paper, published earlier this week in Frontiers in Marine Science, was authored by three graduate students at the University of Hawaii at Manoa and two co-researchers at the Pacific Whale Foundation.

“We expected to see critical warming in some of the breeding grounds, but the number of critically affected areas was a surprise,” said Hannah von Hammerstein, one of the co-authors, in a statement that accompanied the study’s publication.

But the findings were not hopeless. The research also showed that in a “middle of the road” scenario, in which nations cut emissions to a more moderate level, only 35\% of current breeding grounds would become too hot by 2100.

“While the results of the study are daunting, they also highlight the differences between the two emission scenarios and what still can be won by implementing emission mitigation measures,” said von Hammerstein, a graduate student in geography and environment.

“Our findings provide yet another example of what is to come with anthropogenic climate change, with humpback whales representing merely one impacted species,” said the paper’s co-author Martin van Aswegen, a graduate student in marine biology.

World
Qatar's emir in Cairo for 1st time since Arab spat resolved
[title]

CAIRO (AP) — Qatar’s emir arrived in Cairo late Friday for talks with Egypt's president, his first visit to the country following years of frayed ties and a boycott of Doha by four Arab states, including Egypt.

With Qatari and Egyptian flags flowing over the tarmac, Sheikh Tamim bin Hamad Al Thani was greeted at the airport by President Abdel Fattah el-Sissi, a courtesy only granted to leaders of heavyweight allies.

The two were expected to discuss on Saturday key regional issues ahead of President Joe Biden’s anticipated trip to the Middle East next month and to deliberate on ways to further improve bilateral diplomatic and economic relations, local media reported.

The emir's visit came less than two months after his government announced that it would invest \$5 billion in Egypt, another lifeline to the country's economy which has been dealt a blow following the Russian invasion of Ukraine. The announcement came during a March visit by Qatar Foreign Minister Mohammad bin Abdulrahman.

Egyptian-Qatari relations deteriorated in 2013, when Egypt's military removed from power the Islamist President Mohamed Morsi, who was backed by Qatar, and cracked down on his Muslim Brotherhood.

Doha, Qatar's capital, eventually became a haven for fleeing Egyptian Islamists, and the state-owed Qatari broadcaster Al Jazeera Television took a decided stance against el-Sissi's government.

In 2017, Egypt joined Saudi Arabia, the United Arab Emirates and Bahrain in a boycott of Qatar in an effort to force Doha to change its policies. With a wide-ranging trade embargo, a ban on Qatar-bound flights from their airspace and a media blitz, they called on Doha to end close relations with Turkey, Iran and Islamists across the region.

Qatar rejected the quartet’s demands, which included that it shutter its Al Jazeera news network, expel a small contingency of Turkish troops from its territory and cut ties with the Muslim Brotherhood. It also denied claims by the quartet that it supports extremists.

The boycott pushed the gas-rich nation in closer alliance with Turkey and Iran while Doha also continued to strengthen ties with Washington.

The rift finally ended in 2021, when Qatar signed a declaration with the four to normalize relations. Since then, ties have improved and top officials have exchanged visits.

El-Sissi also met with the emir in November, on the sidelines of the climate change summit in Glasgow, and most recently in February, when they both attended the opening of the Winter Olympics in Beijing. Photographs of the two from the events warmly shaking hands came as early signs of renewed rapport.
UK Plan to Override Brexit Deal Passes Hurdle With Tory Dissent
[title]

Boris Johnson’s bill to override the Brexit deal he negotiated survived a challenge in the House of Commons from opponents in the prime minister’s own Conservative Party -- including his immediate predecessor, Theresa May -- as members of Parliament voted to allow it to proceed to the next legislative step.

MPs voted by 295 to 221 to allow the Northern Ireland Protocol Bill to pass its second reading in the Commons, meaning it now progresses to the so-called committee stage, when the text will be considered line-by-line and amendments will be considered.

But the debate exposed the fractures that remain over EU relations within Johnson’s Tories, as MPs including May, former International Development Secretary Andrew Mitchell and Northern Ireland Select Committee Chairman Simon Hoare panned the proposal, saying it broke international law and damaged the UK’s reputation.

“I cannot support it,” May said. “It will diminish the standing of the United Kingdom in the eyes of the world.”

The timing was particularly awkward for Johnson as he met European Union leaders at the Group of Seven summit in Germany. His plan would allow Britain to unilaterally amend the post-Brexit settlement for Northern Ireland, risking a trade war with the EU.

The legislation has provoked renewed legal action from the EU and soured relations with the UK’s biggest trading partner. Speaking at the G-7 on Monday, Johnson told reporters his proposal could be carried out “fairly rapidly” and he wants it done by year-end.

“We could do it very fast, Parliament willing,” Johnson said.

But the bill could take as long as a year to pass Parliament and become law if the upper House of Lords digs in.

Johnson’s government argues the legislation is necessary to address disruption to trade caused by the Brexit deal it signed, which created an effective customs border between Northern Ireland and mainland Great Britain. It also wants to restore the region’s power-sharing executive, which has collapsed due to the Democratic Unionist Party’s opposition to the protocol.

‘Failure of Statecraft’

Foreign Secretary Liz Truss said on Monday that ministers had to proceed with the plan because the EU isn’t being sufficiently flexible in negotiations and won’t agree to change the text of the protocol.

“We simply cannot allow this situation to drift,” Truss said, insisting the plan is legal. The bill will “fix the practical problems the protocol has created.”

The changes the UK government wants to make to the protocol include reducing customs paperwork for traders sending goods across the Irish Sea, stripping the European Court of Justice of its role in settling disputes and extending UK subsidy controls and tax breaks to Northern Ireland.

Legal experts have widely criticized the position as being in breach of international law, a claim that was also made by the dissenting Tory MPs. Hoare called the plan a “failure of statecraft” and said the arguments for it are “flimsy at best and irrational at worst.” Mitchell said the move “trashes our international reputation” and “threatens a trade war when our economy is flat.”

‘Uncertainty’

An EU trade war is a prospect because the bloc says the post-Brexit trade agreement is conditional on Britain respecting the terms of their divorce, of which the so-called Northern Ireland protocol was a key part.

The EU’s chief Brexit negotiator, Maros Sefcovic, told reporters during a trip to Oslo on Monday that the UK plans mean “constant uncertainty.”

“What we are communicating to our UK partners is ‘come back to the negotiating table, respect international law,’” he said. “Because if the bill would be adopted as drafted, we simply have to keep all options on the table.”

U.S.-Iran nuclear negotiations in Qatar end without breakthrough
[title]

Indirect talks between Iran and the U.S. have ended in Doha, Qatar, with no sign of a breakthrough in efforts to revive a 2015 nuclear deal, raising the risk of a potential confrontation with Tehran in coming months.

“Unfortunately, not yet the progress the EU team as coordinator had hoped-for. We will keep working with even greater urgency to bring back on track a key deal for non-proliferation and regional stability,” European Union envoy Enrique Mora tweeted, calling the discussions “intense.”

Mora was the intermediary in the Qatari capital between Iranian chief negotiator Ali Bagheri Kani and President Joe Biden’s special envoy, Rob Malley, passing messages back and forth between the two sides. Iran has refused to hold direct talks with the U.S. team.

The 2015 nuclear deal, known as the Joint Comprehensive Plan of Action, or JCPOA, was designed to prevent Iran from developing nuclear weapons. Former President Donald Trump pulled the U.S. out of the JCPOA in 2018, and the Biden administration has been trying to revive it.

But with the prospects for salvaging the agreement looking increasingly bleak, the Biden administration is coming under growing pressure in Washington and from Middle Eastern allies to consider other options to counter Iran’s nuclear program, former officials, congressional aides and analysts said.

At the request of senators two weeks ago, the Biden administration provided a closed-door classified briefing on Iran, laying out possible “Plan B” options if diplomacy fails to rescue the 2015 nuclear deal, lawmakers said. Biden is due to visit Israel and Saudi Arabia next month, and Iran’s nuclear program is expected to be at the top of the agenda.

Iran’s foreign ministry spokesperson, Nasser Kanani, said Wednesday that the talks in Doha were “held in a professional and serious atmosphere” and that the plan from the outset was to hold two days of discussions.

The U.S., however, accused Iran of being the source of the stalemate.

“In Doha, as before, we made clear our readiness to quickly conclude and implement a deal,” a State Department spokesperson said. “Yet in Doha, as before, Iran raised issues wholly unrelated to the JCPOA and apparently is not ready to make a fundamental decision on whether it wants to revive the deal or bury it.”

The spokesperson expressed gratitude to the E.U. for its efforts but said the U.S. was “disappointed that Iran has, yet again, failed to respond positively to the E.U.’s initiative.”

Iran’s U.N. mission did not respond to a request for comment.

Neither side went to the Doha talks with any major new proposals, and there was no sign Iran had eased its negotiating demands, including insisting that the U.S. remove Iran’s Revolutionary Guard Corps from its terrorism blacklist, according to Ali Vaez of the International Crisis Group think tank.

U.S. negotiators previously have made it clear that they view the Revolutionary Guard sanctions as outside the parameters of the 2015 deal and that Iran would need to offer an equivalent concession in return.

Iran also continues to demand that the U.S. offer guarantees that Washington will not pull out of the agreement again as Trump did. But U.S. officials say there is no way to provide that assurance given that elections might produce a different policy under a new U.S. president.

Negotiated during Barack Obama’s administration, the 2015 JCPOA imposed strict limits on Iran’s uranium enrichment work in return for an easing of economic sanctions. When Trump withdrew the U.S. from the deal in 2018, he said that it was too lax and that it failed to address Iran’s missile program or its support of proxies across the Middle East. 

Since the U.S. exit, Iran has steadily surpassed the deal’s restrictions on its uranium enrichment work, building up stockpiles, running advanced centrifuges and blocking full access to the U.N. atomic watchdog agency. Arms control experts say Iran now could quickly produce weapons-grade uranium without being detected by U.N. inspectors.

An Iranian news agency, Tasnim, earlier described the negotiations as having had “no effect on breaking the deadlock in the talks.”

“What prevented these negotiations from coming to fruition is the U.S. insistence on its proposed draft text in Vienna that excludes any guarantee for Iran’s economic benefits,” Tasnim reported, citing informed sources at the talks.

Last year, Secretary of State Secretary Antony Blinken said the U.S. was “prepared to turn to other options” if the nuclear negotiations fail. U.S. officials have suggested the administration would be ready to tighten sanctions against Iran under that scenario.

European diplomats and former U.S. officials have told NBC News that the U.S. would be likely to introduce new sanctions against Iran and seek to more strictly enforce existing sanctions, with a particular focus on targeting Tehran’s oil sales to China. Potential sabotage operations against the nuclear program also could be on the table.
UN urges Libya's rivals to agree on elections this week
[title]

The U.N. political chief urged Libya’s rival factions on Monday to agree on measures governing the transition to elections during talks in Geneva later this week, expressing hope this will lead to long-awaited voting “at the earliest possible date.”

Rosemary DiCarlo told the U.N. Security Council that during talks in Cairo from June 12-20 the rivals reached “a broad consensus on most of the contentious articles” in the proposed 2017 constitution, which she called “commendable.”

Oil-rich Libya has been wrecked by conflict since a NATO-backed uprising toppled and killed longtime dictator Moammar Gadhafi in 2011. The country was then split by rival administrations, one in the east, backed by military commander Khalifa Hifter, and a U.N.-supported administration in the capital of Tripoli. Each side is supported by different militias and foreign powers.

The Cairo meeting was the first to see Libya’s east-based parliament, the House of Representatives, and west-based High Council of State in Tripoli engage in “a serious review” of the constitutional proposal since its adoption in 2017, DiCarlo said.

“We are encouraged that the leaders of both chambers have accepted the invitation of (U.N.) special adviser Stephanie Williams to meet in Geneva from June 28-29 to discuss and reach agreement on the measures governing the transitional period leading to elections,” she said.

DiCarlo urged the Security Council’s 15 member nations and all of Libya’s international partners “to call on the leadership of the two chambers to seize the opportunity presented by the agreement reached in Cairo” and “make elections happens.”

Libya’s plan for elections last Dec. 24 fell through after the interim administration based in Tripoli, headed by Prime Minister Abdul Hamid Dbeibah, failed to go ahead with the vote. The failure was a major blow to international efforts to end a decade of chaos in Libya.

Dbeibah refused to step down, raising questions over his mandate. In response, the country’s east-based lawmakers elected a rival prime minister, Fathy Bashagha, a powerful former interior minister who is now operating a separate administration out of the city of Sirte.

The rival administrations are now claiming power, after tentative steps toward unity last year.

DiCarlo called for national reconciliation efforts, warning that “continued political divisions are contributing to a tense security environment in and around Tripoli.”

The issue of Libya’s chief executive has not been resolved and she warned that as armed group position themselves to support Debebah or Bashagha “the risk of escalation increases.”

After the recent Cairo meeting, Libyan media reports claimed that the main contested topic was the criteria for a presidential candidacy.

According to the reports, the Tripoli-based council insisted on banning military personal from running for the country’s top post — apparently a move directed at Hifter, a divisive military leader who announced his bid to run in December's elections, while the east-based lawmakers called for allowing military personnel to run.

Fertiliser shortage hits African farmers battling food crisis
[title]

Under the beating Tanzanian sun, Lossim Lazzaro nervously looks over his farm.

He slowly pours livestock manure on his crops, in a last-ditch attempt to help them grow.

Mr Lazzaro owns five acres of land and was once a successful tomato farmer in the northern Arusha region. But now, like many others, he is battling to keep his business and crops alive, amid a global fertiliser shortage.

"It's been difficult for me to get fertiliser in the market," Mr Lazzaro says.

Fertiliser - the key ingredient needed to help crops grow - is in short supply across the world. Global prices have also sky-rocketed in part because of the Russia-Ukraine conflict.

"I used to buy fertiliser for about \$25 (£20) per 50 kg bag in 2019," Mr Lazzaro recalls.

"But the same bag now goes for almost double that price. It is extremely expensive for me."

The amount of fertiliser available globally has almost halved, while the cost of some types of fertilizer have nearly tripled over the past 12 months, according to the United Nations.

That is having a knock-on effect in countries like Tanzania, where farmers are dependent on imported fertiliser.

"I ended up buying fertiliser from a local manufacturer but still I have to place an order months earlier due to the shortage," Mr Lazzaro adds.

The crisis is fuelling fears of food scarcity.

Africa - which already uses the least amount of fertiliser per hectare in the world - is at high risk.

The short supply will inevitably impact crop yields, particularly for wheat which requires a lot of fertiliser and is essential for feeding millions.

The World Food Programme (WFP) has warned that the fertiliser shortage could push an additional seven million people into food scarcity.

They say that cereal production in 2022 will decline to about 38 million tonnes, from the previous year's output of over 45 million tonnes.

Tanzania, like many other African countries, relies on fertiliser from Russia and China - the two leading global manufacturers.

Russia, which is under Western sanctions, produces large amounts of potash, ammonia and urea.

These are the three key ingredients needed to make chemical fertiliser. They helped to fuel the Green Revolution in the 1960s which tripled global grain production and helped to feed millions.

Russia exports around 20\% of the world's nitrogen fertilisers and combined with its sanctioned ally Belarus, 40% of the world's exported potassium, according to data from Rabobank.

The cost of fertiliser was already high following the economic fallout of the Covid-19 pandemic. Now, the sanctions on Russia and Belarus, compounded with export controls in China, have made a bad situation worse.

The crisis has left many African countries, which are heavily dependent on foreign imports, scrambling to find solutions.

Demand for locally produced fertiliser is rising. Small-scale farmers in the north of Tanzania are now turning to places like Minjingu Mines and Fertilizer Ltd, one of the biggest fertiliser manufacturers in the country.

The company says it is experiencing a sudden increase in demand and is struggling to fill orders. But bosses say they are unable to increase their capacity due to heavy taxation.

"We don't have a level playing ground compared to the importers," said Tosky Hans, a director of Minjingu Mines and Fertilizer.

"Local manufacturers have to pay a lot of taxes, whereas the importers don't," he added.

Like many other countries, foreign investors are given subsidies in Tanzania to attract investment while local manufacturers pay set taxes.

Alliance for Green Revolution in Africa (Agra), a non-government organisation that promotes green solutions across the continent, says this is an opportunity for farmers to become more self-sufficient.

Vianey Rweyendela, country manager of Agra Tanzania, encourages farmers to unionise and form cooperatives. A move he says that could give them a voice on market prices.

"That will help them have bargaining power and fertiliser sold to them will be affordable," argues Mr Rweyendela.

The richest man in Africa, Aliko Dangote, recently commissioned a fertiliser plant in Nigeria, which is expected to produce three million tonnes of urea fertiliser annually.

He believes, guaranteed supplies will make the difference.

"Ordering fertiliser and having it arrive has been a big challenge for farmers in Africa and they end up missing their planting season," said Mr Dangote.

"With the launch of this plant, we shall ensure farmers get the nutrients early."
COVID-19
Deadline passes and 1 in 10 Army National Guard soldiers still unvaccinated for Covid. Will they be expelled?
[title]

The deadline for all Army National Guard soldiers to be vaccinated for Covid passed at midnight, with about a tenth of the 330,000 soldiers still unvaccinated and subject to financial penalties or potential future expulsion.

Defense officials, however, said that amid the Guard's recruiting crisis, there are already signs that unit commanders may be allowed to let unvaccinated troops continue receiving pay and benefits for some period.

In November, Secretary of Defense Lloyd Austin directed that members of the Army National Guard and the Air National Guard who were unvaccinated by the deadline would be unable to participate in drills, get paid or put their service days toward their retirement. Their continued refusal could result in "separation," or expulsion from the service.

About 14,000 members of the Army Guard have explicitly refused to be vaccinated. Another 7,000 have requested exemptions, many for religious reasons, the officials said.

Prior to publication of this article, the Army did not answer questions about whether it would enforce the threat of separation. On Monday, NBC News reported that every branch of the U.S. military is struggling to meet its 2022 recruiting goals.

As of June 27, 86.4\% of Army Guard soldiers were fully vaccinated and 88.59\% had received at least one dose of the vaccine. The Army Guard has about 330,000 total members, meaning that more than 37,000 had not been vaccinated as of Monday.

The Army will release new figures for total vaccinations Friday. It is also scheduled to begin enforcing the vaccination requirement Friday.

According to defense officials, however, because of the fear of losing troops in a bad year for recruiting, individual unit commanders may be allowed to put unvaccinated troops in a temporary status that would let them keep their pay and benefits longer,

The officials say that if the unvaccinated troops have requested an exemption, have begun vaccination but not entered their information into the military's electronic health record, or if they are being processed for separation, commanders can assign them to a temporary duty status that allows them to be paid and earn retirement credit, potentially for months, while they complete their administrative processes.

Overall, about 90\% of the total 435,000 National Guard service members — both the Air Guard and the Army Guard — are now vaccinated, according to National Guard officials. About 94% of the Air Guard members are vaccinated.

Defense officials are hopeful some of the more than 37,000 Army Guard holdouts will get their vaccine and not be forced out.

“We’re going to give every soldier every opportunity to get vaccinated and continue their military career,” said Lt. Gen. Jon Jensen, director of the Army Guard. “We’re not giving up on anybody until the separation paperwork is signed and completed.”
US grapples with whether to modify COVID vaccine for fall [~1000 words]
[title]

U.S. health authorities are facing a critical decision: whether to offer new COVID-19 booster shots this fall that are modified to better match recent changes of the shape-shifting coronavirus.

Moderna and Pfizer have tested updated shots against the super-contagious omicron variant, and advisers to the Food and Drug Administration will debate Tuesday if it’s time to make a switch — setting the stage for similar moves by other countries.

“This is science at its toughest,” FDA vaccine chief Dr. Peter Marks told The Associated Press, adding that a final decision is expected within days of the advisory panel's recommendation.

Current COVID-19 vaccines saved millions of lives around the world in just their first year of use. And the Moderna and Pfizer shots still offer strong protection against the worst outcomes -- severe illness and death — especially after a booster dose.

But those vaccines target the original coronavirus strain and between waning immunity and a relentless barrage of variants, protection against infections has dropped markedly. The challenge is deciding if tweaked boosters offer a good chance of blunting another surge when there's no way to predict which mutant will be the main threat.

In an analysis prepared for Tuesday's meeting, FDA officials acknowledged targeting last winter's version of omicron is “somewhat outdated" since it already has been replaced by its even more contagious relatives.

“We would obviously like to get it right enough," Marks said, so that with one more shot “we get a full season of protection.”

Many experts say updated boosters promise at least a little more benefit.

“It is more likely to be helpful” than simply giving additional doses of today’s vaccine, said epidemiologist William Hanage of the Harvard T.H. Chan School of Public Health.

That’s assuming the virus doesn’t throw another curve ball.

“We’re following rather than getting ahead which is so vexing -- that we haven’t come up with a better variant-proof vaccine,” said Dr. Eric Topol, head of the Scripps Research Translational Institute, who has urged a major government push for next-generation immunizations.

Adding to concern about a winter COVID-19 wave is that about half of Americans eligible for that all-important first booster dose never got it. An updated version might entice some of them.

But “we do need to change our expectations,” said Dr. William Moss of the Johns Hopkins Bloomberg School of Public Health, who noted that studies early in the pandemic raised unrealistic hopes of blocking even the mildest infections. “Our strategy can’t be booster doses every couple of months, even every six months, to prevent infections.”

The top candidates are what scientists call “bivalent” shots — a combination of the original vaccine plus omicron protection.

That’s because the original vaccines do spur production of at least some virus-fighting antibodies strong enough to cross-react with newer mutants -- in addition to their proven benefits against severe disease, said University of Pennsylvania immunologist E. John Wherry.

“Being able to push the boost response a little bit in one direction or the other without losing the core is really important,” he said.

Moderna and Pfizer found their combo shots substantially boosted levels of omicron-fighting antibodies in adults who'd already had three vaccinations, more than simply giving another regular dose.

Recipients also developed antibodies that could fight omicron’s newest relatives named BA.4 and BA.5, although not nearly as many. It's not clear how much protection that will translate into, and for how long.

Antibodies are a key first layer of defense that form after vaccination or a prior infection. They can prevent infection by recognizing the outer coating of the coronavirus -- the spike protein -- and blocking it from entering your cells.

But antibodies naturally wane and each new variant comes with a different-looking spike protein, giving it a better chance of evading detection by remaining antibodies. Separate studies published this month in Nature and the New England Journal of Medicine show the newest omicron relatives are even better at dodging antibodies — both in the vaccinated and in people who recovered from the original omicron.

That first booster people were supposed to get strengthened immune memory, helping explain why protection against hospitalization and death is proving more durable. If the virus sneaks past antibodies, different defenders called T cells spring into action, attacking infected cells to curb illness.

“T cells recognize the virus in a fundamentally different way,” not hunting for disguised spike protein but for parts of the virus that so far haven't been altered as much, said Penn’s Wherry.

Still, as people get older, all parts of their immune system gradually weaken. There’s little data on how long T cell protection against COVID-19 lasts or how it varies with different mutations or vaccines.

Wherry and dozens of other scientists recently petitioned the FDA to quit focusing solely on antibodies and start measuring T cells as it decides vaccination strategy.

The Biden administration has made clear that it needs Congress to provide more money so that if the FDA clears updated boosters, the government can buy enough for every American who wants one. And Dr. Anthony Fauci, the government's top infectious disease expert, told Congress last week more research funding also is critical to create better next-generation vaccines, such as nasal versions that might better block infection in the nose or more variant-proof shots.

“The virus is changing and we need to keep up with it,” Fauci, said.
As COVID fears ebb, Japan readies for tourists from abroad [~1000 words]
[title]

The rickshaw men in Tokyo are adding English-speaking staff, a sure sign Japan is bracing for a return of tourists from abroad.

Japan’s border controls to curb the spread of coronavirus infections began gradually loosening earlier this month.

That's great news for Yusuke Otomo, owner of Daikichi, a kimono rental shop in Asakusa, an old district of Tokyo famous for its temples, quaint restaurants and rickshaw rides. He can barely contain his excitement.

“Those were a hard three years. But we managed to endure until today. And after such an experience, to think people from abroad can finally come back is simply thrilling,” Otomo told The Associated Press.

“I’m thinking that maybe, just as before COVID, my shop, the city of Asakusa and everyone’s hearts can flourish again. I can’t wait.”

Before the pandemic, Asakusa was so brimming with foreigners they sometimes outnumbered the Japanese. After the coronavirus struck, the streets were deserted.

“Not a soul in sight,” he said sadly.

Some kimono rental stores folded. Restaurants were shuttered.

The crowds are finally back with a gradual relaxing of the city's COVID-19 restrictions, which called for restaurants to close early and people to social distance and limit attendance at events. But most of the visitors are Japanese.

Shuso Imada, general manager at JSS Information Center, a sake and shochu showroom in downtown Tokyo, said he has been feeling pretty lonely and is itching to tell foreign visitors about how to match the traditional Japanese rice wine with all kinds of non-Japanese food, even cheese and beef.

“In a way, we didn't have much to do and we just had to wait. The gates have now reopened,” he said.

But like others waiting for tourists, he acknowledged that the limited entry for tour groups now in effect may not allow time for a relaxing visit to his center.

Visitors have to abide by guidelines requiring travelers to have a special coordinator, stay on specific routes and abide by rules like wearing masks and regularly using disinfectant.

Before COVID, tourism was booming as a mainstay of Japan's economy, the world's third largest. Foreign visitors numbered a record 32 million in 2019 and the target for 2020 was 40 million. After COVID struck, the government gradually imposed very restrictive limits on foreign arrivals, for a time excluding many foreign residents.

As of June 10, it is allowing foreign tourists to visit, but in limited numbers and only on group tours, not as individual travelers.

Visas are required for nearly everyone, even those from countries that normally would have visa-free entry. And they're available only to travelers from 98 so-called “blue” countries, including the U.S., who are deemed to pose a minimal health risk and can enter without a quarantine if they show proof they tested negative for COVID within 72 hours of their departures.

People entering Japan from countries considered to be a greater risk must quarantine for three days at home or in government-designated facilities. There is a daily cap on arrivals of 20,000 people, including all travelers. And the number of airports open to foreign tourists also is gradually expanding.

Worries about COVID-19 remain. If infections shoot up again in another wave, pandemic precautions could be brought back.

Japan, a crowded island nation, is wary about outside risks and infectious diseases. After about two years of seeing very few tourists, Japanese have some adjusting to do, Otomo and others said.

So the authorities are taking it slow.

“I would love to have tourists from abroad come, as long as everyone, including myself, abides by the rules, like wearing masks and keeping sanitary standards,” said Minaho Iwase, who was visiting Tokyo from Aichi, central Japan, recently.

Many tourists might be deterred by the restrictions on independent travel. But some seem not to mind.

“When my friends asked me to join this trip to Japan, I immediately said, ‘Yes.’ I visited Japan before. I love their food, their tradition, and their highly organized culture. Japan is great,” said Sorrasek Thuantawee, an office worker who joined a group of eight Thais excitedly preparing to board a flight from Bangkok last week.

Japan is a favorite destination, despite its not "opening up 100%," said Nuttavut Mitsumoto, the guide for the group, Thai travel agency Compax World’s first to Japan since it relaxed its entry rules.

The Japanese yen has weakened this year against the U.S. dollar and other currencies, making visits something of a bargain.

A study last month by Money.co.uk, a free online service that compares financial products, found Osaka ranked fourth and Tokyo eighth for most affordable “luxury travel,” including Michelin star meals and five-star hotels.

Back in Asakusa, rickshaw man Shunpei Katayama has yet to drive around his first post-COVID foreign tourist, but English-speaking drivers are back on the job. And for now, Japanese visitors from outside Tokyo are keeping him busy.

“Japanese who can’t go to Guam and other spots abroad come visit Shibuya. And Asakusa,” he said.

On a recent day, Otomo was shooting photos of a Japanese mother and daughter dressed up in colorful kimono to attend a friend’s wedding in Tokyo.

The foreign clientele that used to frequent his shop were so enthusiastic about dressing up as samurai, ninja and geisha, complete with swords and hair ornaments. Some quickly became friends, regardless of their nationalities, Otomo recalled a bit sentimentally.

“When they’re happy, I’m happy. They get my adrenaline going,” he said.
COVID vaccines saved 20M lives in 1st year, scientists say
[title]

Nearly 20 million lives were saved by COVID-19 vaccines during their first year, but even more deaths could have been prevented if international targets for the shots had been reached, researchers reported Thursday.

On Dec. 8, 2020, a retired shop clerk in England received the first shot in what would become a global vaccination campaign. Over the next 12 months, more than 4.3 billion people around the world lined up for the vaccines.

The effort, though marred by persisting inequities, prevented deaths on an unimaginable scale, said Oliver Watson of Imperial College London, who led the new modeling study.

“Catastrophic would be the first word that comes to mind,” Watson said of the outcome if vaccines hadn't been available to fight the coronavirus. The findings “quantify just how much worse the pandemic could have been if we did not have these vaccines."

The researchers used data from 185 countries to estimate that vaccines prevented 4.2 million COVID-19 deaths in India, 1.9 million in the United States, 1 million in Brazil, 631,000 in France and 507,000 in the United Kingdom.

An additional 600,000 deaths would have been prevented if the World Health Organization target of 40% vaccination coverage by the end of 2021 had been met, according to the study published Thursday in the journal Lancet Infectious Diseases.

The main finding — 19.8 million COVID-19 deaths were prevented — is based on estimates of how many more deaths than usual occurred during the time period. Using only reported COVID-19 deaths, the same model yielded 14.4 million deaths averted by vaccines.

The London scientists excluded China because of uncertainty around the pandemic’s effect on deaths there and its huge population.

The study has other limitations. The researchers did not include how the virus might have mutated differently in the absence of vaccines. And they did not factor in how lockdowns or mask wearing might have changed if vaccines weren’t available.

Another modeling group used a different approach to estimate that 16.3 million COVID-19 deaths were averted by vaccines. That work, by the Institute for Health Metrics and Evaluation in Seattle, has not been published.

In the real world, people wear masks more often when cases are surging, said the institute's Ali Mokdad, and 2021's delta wave without vaccines would have prompted a major policy response.

“We may disagree on the number as scientists, but we all agree that COVID vaccines saved lots of lives," Mokdad said.

The findings underscore both the achievements and the shortcomings of the vaccination campaign, said Adam Finn of Bristol Medical School in England, who like Mokdad was not involved in the study.

“Although we did pretty well this time — we saved millions and millions of lives — we could have done better and we should do better in the future," Finn said.

Funding came from several groups including the WHO; the UK Medical Research Council; Gavi, the Vaccine Alliance; and the Bill and Melinda Gates Foundation.
Should you get a COVID-19 booster shot now or wait until fall? Two immunologists help weigh the options [~1000 words]
[title]

While COVID-19 vaccines continue to be highly effective at preventing hospitalization and death, it has become clear that the protection offered by the current vaccines wanes over time. This necessitates the use of booster shots that are safe and effective in enhancing the immune response against the virus and extending protection.

But when to get a first or second booster, and which shot to choose, are open questions. Many people find themselves unsure whether to wait on new, updated formulations of the COVID-19 vaccines or to mix and match combinations of the original vaccine strains.

SARS-CoV-2, the virus that causes COVID-19, uses its knob-shaped spike protein to gain entry into cells and to cause infection. Each of the existing and upcoming vaccines relies on emulating the spike protein to trigger the immune response. However, each vaccine type presents the spike protein to the immune system in different ways.

As immunologists studying inflammatory and infectious diseases, including COVID-19, we are interested in understanding how the COVID-19 vaccine designs differ in the type of immunity they trigger and the protection that results.

New bivalent vaccines
Moderna and Pfizer-BioNTech, the two companies whose mRNA vaccines have been the primary options for COVID-19 vaccination across all age groups, both have new vaccine formulations on the way. An advisory committee of the Food and Drug Administration is set to meet on June 28, 2022, to evaluate the newest versions and to decide on which are likely to be recommended for use in this fall’s booster shots.

Moderna’s new bivalent vaccine mixes mRNA that encodes for the spike proteins of the original SARS-CoV-2 virus as well as the slightly different spike protein of the more infectious omicron variant.

In early June 2022, Moderna said that in clinical trials, its bivalent vaccine outcompetes the original vaccine strain, inducing a stronger immune response and longer protection against the original SARS-CoV-2 and its variants, including omicron.

Moderna later announced that its newest formulation also performs well against the newest omicron subvariants, BA.4 and BA.5, which are quickly becoming the dominant strains in the U.S. Because of the significantly stronger immune response that the new shot induces, Moderna predicts that such protection may last a year and plans to introduce its new vaccine in August.

And most recently, on June 25, Pfizer-BioNTech also announced results for its two new COVID-19 vaccine formulations: a bivalent formulation consisting of mRNA that encodes for the spike proteins of the original SARS-CoV-2 strain and the original BA.1 omicron subvariant, and a “monovalent” version that is only directed at the spike protein of BA.1.

The company’s preliminary studies demonstrated that both the monovalent and the bivalent vaccines triggered antibodies that neutralized the newer omicron BA.4 and BA.5 subvariants, although to a lesser degree than the BA.1 subvariant. However, Pfizer’s monovalent vaccine triggered better virus-neutralizing antibodies against the omicron BA.1 subvariant than did the bivalent vaccine.

However, whether the differences in the levels of such antibodies seen with the monovalent versus bivalent vaccines translate into different levels of protection against newer omicron variants remains to be established in clinical trials.

Progress on the Novavax vaccine
Another vaccine formulation that is working its way toward authorization is Novavax, a vaccine built using the spike protein of the original SARS-CoV-2 virus. The Novavax vaccine has the advantage of being similar to traditional vaccines, such as the DTaP vaccines against diphtheria, tetanus and pertussis, or the vaccines against other viral infections such as hepatitis and shingles. The Novavax vaccine has been clinically tested in South Africa, the United Kingdom and the U.S. and found to be safe and highly effective with 90% efficacy against mild, moderate and severe forms of COVID-19.

An advisory committee to the Food and Drug Administration endorsed the Novavax vaccine in early June 2022. Now, the FDA is reviewing changes that Novavax made during its manufacturing process before making its decision to authorize the shot.

In Australia, the Novavax vaccine was recently registered provisionally as a booster for individuals aged 18 years and over. The company is performing phase 3 clinical trials to determine if its vaccine can be used safely and effectively as a booster in people who have previously taken mRNA vaccines.

When these new vaccines become available in the coming months, people will have significantly more options for mixing and matching vaccines in order to enhance the duration and quality of their immune protection against COVID-19.

Mixing and matching
Until then, clinical studies have shown that even mixing and matching the existing vaccine types is an effective strategy for boosting. For example, recent studies suggest that when adults who were fully vaccinated with any of the original three COVID-19 vaccines – Pfizer-BioNTech, Moderna or Johnson & Johnson – received a booster dose with a different vaccine brand from the one they received in their initial series, they had a similar or more robust immune response compared to boosting with the same brand of vaccine.

Vaccine mixing has been found to be safe and effective in various studies. The reason why mixing vaccines might produce a more robust immune response goes back to how each one presents the spike protein of the virus to the immune system.

When the SARS-CoV-2 virus mutates in regions of the spike protein, as has been the case with each of the variants and subvariants, and tries to evade the immune cells, antibodies that recognize different parts of the spike protein can stop it in its tracks and prevent the virus from infecting the body’s cells.

So whether you decide to get a booster shot now or wait until the fall, for many it’s heartening to know that more options are on the way.
Climate Change
'Moment of reckoning:' Federal official warns of Colorado River water supply cuts
[title]

The Colorado River’s reservoirs have diminished to the point that significant cuts to the water supplied to the seven states that rely on it will be necessary next year, a federal official warned Tuesday.

Bureau of Reclamation Commissioner Camille Calimlim Touton told the Senate Energy and Natural Resources Committee maintaining “critical levels” at the largest reservoirs in the United States — Lake Mead and Lake Powell — will require large reductions in water deliveries.

“A warmer, drier West is what we are seeing today,” she said at a hearing. “And the challenges we are seeing today are unlike anything we have seen in our history.”

Colorado, New Mexico, Utah, Wyoming, Arizona, California, and Nevada all receive water from the Colorado River and next year will see a decrease of between 2 million and 4 million acre-feet of water due to the ongoing drought that has gripped most of the Western U.S. (An acre-foot is the amount of water needed to cover one acre of land in one-foot-deep water.) Current allotments of water from the Colorado range from 300,000 acre-feet for Nevada to 4.4 million acre-feet for California.

“What has been a slow-motion train wreck for 20 years is accelerating, and the moment of reckoning is near,” John Entsminger, general manager of the Southern Nevada Water Authority, told the Senate hearing. “We are 150 feet from 25 million Americans losing access to the Colorado River, and the rate of decline is accelerating.”

The West has been suffering through an acute drought since 2020, part of a megadrought that began in 2000. The last 20 years have been the driest two decades in the last 1,200 years. This year is so far the driest on record in California. Scientists attribute these conditions to climate change, which causes more water evaporation due to warmer temperatures.

“As a climate scientist, I’ve watched how climate change is making drought conditions increasingly worse — particularly in the western and central U.S.,” wrote Imtiaz Rangwala, research scientist in climate at the Cooperative Institute for Research in Environmental Sciences at the University of Colorado Boulder, in May. “The last two years have been more than 2 degrees Fahrenheit (1.1 Celsius) warmer than normal in these regions. Large swaths of the Southwest have been even hotter, with temperatures more than 3 F (1.7 C) higher.”

Western states have already been undertaking emergency measures to deal with the water scarcity. Seven months ago, California, Arizona and Nevada signed an agreement to take less water from Lake Mead, and six weeks ago the Department of Interior announced it is withholding some water from Lake Powell. Otherwise, DOI feared, the reservoir could drop so low that Glen Canyon Dam would not be able to generate electricity.

Last year, for the first time ever, the federal government declared a shortage on the river, which led to reductions in water deliveries to Arizona and Nevada. Some farmers in Arizona have had to leave some fields unplanted as a result.

Local governments and water utilities have been imposing restrictions on water usage. On June 1, the Metropolitan Water District of Southern California instituted limits on outdoor watering; typically it will be restricted to one or two days per week. But the water shortage persists.

“Despite those efforts and a previous deal among the states to share in the shortages, the two reservoirs stand at or near record-low levels,” the Los Angeles Times reported. “Lake Mead near Las Vegas has dropped to 28% of its full capacity, while Lake Powell on the Utah-Arizona border is now just 27% full.”

Touton told the Senate committee that her agency is negotiating with the seven states that depend on the Colorado River to develop a plan for apportioning the water supply reductions in the next two months. In all, nearly 40 million people rely on water from the river.

Sen. Martin Heinrich, D-N.M., attributed the gathering crisis to a lack of coordinated action to mitigate climate change.

“It’s frankly a direct result of the lack of action on climate that we have seen for more than 20 years,” Heinrich said.
It's not summer yet, but climate change is already showing its teeth in 2022 [~1000 words]
[title]

The evidence of how climate change is already affecting our world seems to grow more pronounced with every passing day.

At least 2,000 cows at a Kansas feedlot were killed this week by excessively high temperatures, as the latest record-breaking spring heat wave pushed east across the country.

“This was a true weather event — it was isolated to a specific region in southwestern Kansas," A.J. Tarpoff, a cattle veterinarian with Kansas State University, told the Associated Press. “Yes, temperatures rose, but the more important reason why it was injurious was that we had a huge spike in humidity ... and at the same time, wind speeds actually dropped substantially, which is rare for western Kansas.”

On Wednesday, the National Weather Service advised more than one-third of the U.S. population to remain indoors to protect themselves against that same potentially deadly combination of heat and humidity. Scientists have termed that lethal mix the "wet-bulb" effect. When the body gets hot, it sweats, and the evaporation of that sweat helps cool the body. But when the humidity in the atmosphere is too high, that evaporation isn't possible, and the sweat doesn't help cool the body down.

“We need a differential between the human body and the environment, and if the air is already holding as much moisture as it can, you don't have that gradient,” Radley Horton, Lamont Research Professor at Columbia University’s Lamont-Doherty Earth Observatory, told Vice News. “Your body's not able to get the atmosphere to take that moisture from it.”

While climate scientists had previously predicted that such high temperatures and humidity would not arrive on Earth until the mid-21st century, recent studies have found that "extreme humid heat overall has more than doubled in frequency since 1979."
Dozens of logs ripped from their roots are trapped around a washed-out bridge in a muddy river.
Logs pile up on a washed-out bridge near Rescue Creek in Yellowstone National Park on June 13. (National Park Service via Getty Images)

On Monday, 10,000 visitors to Yellowstone National Park had to be evacuated after an excess of rainfall unprecedented for June. Roads, bridges and homes in the park were washed away, the park remains closed, and on Thursday, President Biden issued federal disaster assistance to Montana.

The rain unleashed on Montana was part of a so-called atmospheric river that broke records in Washington state shortly before it pushed east. Studies have linked an increase in those records to rising air and water temperatures caused by climate change.

More generally, research has linked rising global temperatures to higher levels of atmospheric moisture, what's known as the Clausius-Clapeyron relation. When conditions are right, that excess moisture is released, causing severe downpours and storms like the ones that hit the Midwest this week, knocking out power to half a million people amid triple-digit temperatures, and making the need for air conditioning acutely felt.

Meanwhile, the extreme drought that has gripped the American West continues apace. The last 20 years have been the driest two decades in the past 1,200 years. As a result, rivers, lakes and reservoirs are drying up at alarming speed.

The Senate Energy and Natural Resources Committee held a hearing this week on the dwindling water supply in the Colorado River and its reservoirs, including Lake Mead and Lake Powell. In all, 40 million people across the West rely on the Colorado for water.
An aerial view of a riverbed now covered in vegetation and the dried-out tributaries that once fed into it.
The arid desert Southwest near Moab, Utah, viewed from 33,000 feet on May 19. (George Rose/Getty Images)

“What has been a slow-motion train wreck for 20 years is accelerating, and the moment of reckoning is near,” John Entsminger, general manager of the Southern Nevada Water Authority, testified at the hearing. “We are 150 feet from 25 million Americans losing access to the Colorado River, and the rate of decline is accelerating.”

Water-rationing restrictions have been put in place in California and are likely to be extended there and in other states in the coming months.

The science is crystal clear about why these weather-related disasters continue to pile up: Human beings are pumping greenhouse gases like carbon dioxide into the atmosphere, which traps the sun's radiation, warming temperatures.

For years now, the Scripps Institute of Oceanography at the University of California, San Diego, has measured that buildup at the Mauna Loa Observatory in Hawaii, charting the steady rise on a graph known as the Keeling Curve.

Ultimately, researchers say, until mankind reduces the amount of carbon dioxide in the atmosphere, the consequences being witnessed this spring will persist. Just as certainly, they will worsen along with the rise of atmospheric carbon dioxide.

Yet there is still much that we don't know about how climate change will play out in the coming decades. A study published in April in the Cornell University astrophysics journal arXiv concluded that mankind is ushering in an unprecedented shift in the Earth's climate system. Those changes, contrary to the claim of Rep. Marjorie Taylor Greene, R-Ga., earlier this week, are not likely to prove "healthy for us."

"The implications of climate change are well known (droughts, heat waves, extreme phenomena, etc)," researcher Orfeu Bertolami told Live Science in an email. "If the Earth System gets into the region of chaotic behavior, we will lose all hope of somehow fixing the problem.”
Leaf blowers, lawn mowers and fertilizer: How lawns contribute to climate change [>1000 words]
[title]

Americans are in love with — or, some might say, addicted to — their lawns. The neatly manicured, bright green plots of grass are ubiquitous in most suburbs, where a majority of Americans live. At least 40 million acres in the United States, an area larger than the state of Georgia, are covered by turf grass, the standard lawn plant.

But what if growing and grooming that grass is contributing to the biggest environmental crises on the planet, including water pollution and climate change?

That’s the view of a number of scientists who are increasingly vocal about the drawbacks of lawns and the need to switch to alternatives — or, at a minimum, more sustainable means of managing one’s lawn.

“There are four things every piece of land needs to be doing if we’re going to reach ecological sustainability: sequester carbon, support pollinators, support a food web. And the other is to manage the watershed. A lawn is the worst choice in all of those four ecological goals,” Douglas Tallamy, a professor of agriculture and natural resources at the University of Delaware, told Yahoo News.

For climate change, the single biggest problem is not what a lawn does, but what it doesn’t do. Every plant stores carbon dioxide — the most widespread heat-trapping gas that is causing global warming. The more carbon that’s stored, the better it is for the environment. But not all plants store the same amount of carbon. Broadly speaking, the amount of carbon sequestered correlates to the size of a plant and its root system. That’s why logging old-growth trees, which tend to be taller than younger trees, is particularly bad for climate change.

Compared to other plants that could grow in a yard, like bushes and trees, lawn grass has a very shallow root system. Much less of it grows above ground, especially if you cut your grass every week to keep it neat and short. “In terms of carbon sequestration, lawns fail,” said Tallamy, the author of “Nature's Best Hope: A New Approach to Conservation That Starts in Your Yard.”

Then there’s the lawn maintenance and machinery that many Americans use to cut and clean their lawns: gas-powered lawn mowers and leaf blowers. According to the Environmental Protection Agency, gas-powered lawn mowers use 800 million gallons of gasoline — and spill an additional 17 million additional gallons of oil — every year. The two-stroke engines used by lawn mowers and leaf blowers are especially dirty because they do not combust about 30% of the fuel they use, which releases volatile organic compounds.

A 2014 study found an idling scooter with a two-stroke engine releases 124 times as much volatile organic compounds as an idling car or truck. The EPA states that using a typical gas-powered lawn mower produces as much volatile organic compounds and nitrogen oxide — a powerful greenhouse gas — as driving 11 average new cars over the same timeframe. In total, according to the agency, lawn mowers account for 5% of American (non-climate) air pollution. On top of that, many lawns are cut by a gardener who visits regularly, burning gasoline on the way there and back.

“Lawns are fossil fuel-dependent, period,” Douglas Kent, a landscape contractor who teaches at Cal Poly Pomona, told Yahoo News. “They don’t have to be, it’s just how we maintain them — the mowers, the blowers, the edgers.”

Then there are the emissions associated with making fertilizer. The most important ingredient in fertilizer is typically ammonia, which contains nitrogen that helps plants grow. Ammonia is made at high pressure and at high temperatures. So it requires a lot of energy, which is usually supplied by fossil fuels like coal and natural gas. Ammonia manufacturing is responsible for more than 1% of global greenhouse gas emissions.

“[Lawns] are huge nitrogen consumers, and nitrogen is the most energy-dense nutrient that we manufacture,” Kent said.

“When you add all that energy we’re dumping in lawns and compare it against the amount of biomass that’s being stored in the soil and the tissue, you come up with 1 acre of lawn [that] contributes approximately 3,112 pounds of carbon dioxide per year, which has the energy equivalent of 156 gallons of gasoline,” Kent added. (He made that calculation, drawing on previous research for the data inputs, for his book, “A New Era of Gardening: A Book on Gardening for Oxygen and a Healthier Atmosphere.”)

Many of the same attributes that make most well-manicured American lawns a net contributor to climate change also cause them to fail Tallamy’s other sustainability tests. Fertilizer, for example, typically comes mixed with herbicide to kill off weeds — the two-in-one products are referred to as “weed and feed.”

But a person’s weed is an insect’s food. The weeds that pollinators depend on, such as clovers and dandelions, are being systematically eliminated from lawns every day. And pollination is the very basis of biodiversity.

“Most vertebrates don't eat plants directly: They eat things that eat the plants, mostly insects,” Tallamy observed.

Likewise, short, regularly cut grass does not absorb much water — an increasingly important task as climate change leads to more flooding from heavier storms — and that runoff can funnel fertilizer and herbicide into lakes, rivers and oceans, potentially poisoning fish and harming swimmers.

“Lawns are destroying our watersheds, because, first of all, they don’t hold the water that other plants are holding,” Tallamy said. “It’s almost like paving the ground during a hot, dry summer.”

Grass is the most prevalent irrigated crop in the U.S., and lawns use 3 trillion gallons of water per year. Due to the warmer temperatures and more severe droughts associated with climate change, water scarcity has become a crisis in much of the West, forcing local governments to limit the amount of water residents can use outdoors, although many homeowners are reportedly ignoring the rules.

To be sure, lawns are not the only detrimental yard features. A concrete patio, which comes with its own carbon emissions from concrete production, has no ecological benefits at all.

So ripping out a lawn and paving it over would not be helpful. But what should you replace it with? Most experts suggest simply reducing the amount of space dedicated to grass and swapping in some bigger plants that will absorb more carbon and water. A tree that provides shade also reduces the amount of water that evaporates from the remaining lawn, meaning that it should require less water.

Ideally, some scientists say, only people living in regions wet enough to grow grass without additional watering would have lawns, and residents of drier regions would plant less thirsty native species, like cactus in the desert.

There are also lower-impact ways of caring for a lawn. Using only manual tools, like a push mower, or electric ones, will remove the emissions from two-stroke engines. According to the Electric Power Research Institute, replacing half of gas mowers in the United States with electric mowers would save as much emissions as taking 2 million cars off the road. Taking a more natural approach to lawn management — cutting it less often, skipping the weed killer and letting the clovers and dandelions grow — would also minimize the impact.

Some state and local governments are beginning to take action on the worst environmental drawbacks of lawns. Responding to complaints about the noise of gas-powered mowers and leaf blowers as much as the emissions, California Gov. Gavin Newsom signed a bill last October that will phase them out in the state.

“Right now, we use [lawn] as a default landscape: We put a few plants in our yard and everything else becomes lawn,” Tallamy said. “I want to turn that on its head. I want to have a lot of plants, and what’s left over becomes lawn.”
U.S. Forest Service admits climate change miscalculation in New Mexico fire
[title]

U.S. Forest Service employees made several mistakes, including underestimating the impact of climate change on conditions in the Southwest, when planning a controlled burn to reduce the threat of wildfires in New Mexico earlier this year, according to a report from the agency released Tuesday.

As a result, the burn exploded into the largest fire in the state’s history, forcing thousands of residents to evacuate their homes.

“Climate change is leading to conditions on the ground we have never encountered,” wrote Forest Service Chief Randy Moore in the foreword to the report. “We know these conditions are leading to more frequent and intense wildfires. Drought, extreme weather, wind conditions and unpredictable weather changes are challenging our ability to use prescribed fire as a tool to combat destructive fires. This spring in New Mexico, a pile burn of hazardous logs that started in January, smoldered underground for months, persisting through multiple snowstorms and freezing temperatures, before resurfacing as a wildfire. That type of event was nearly unheard of until recently in the century-plus of experience the Forest Service has in working on these landscapes.”

After decades of aggressive fire-fighting strategies designed to keep wildfires away from population centers, many U.S. forests have become overgrown, increasing the need for prescribed burns that thin overgrowth and reduce the risk of fire spreading out of control.

“Over the past dozen years, prescribed fire has accounted for an average of 51% of the acreage of hazardous fuels reduction accomplished, or an average of 1.4 million acres per year,” the report noted. “Meeting the objectives of the IIJA [the Infrastructure and Investment Jobs Act] is likely to require the Forest Service to conduct prescribed fires on between 2.5 [million] and 4 million acres annually, nationally.”

A backlog of scheduled prescribed burns dating to Department of Interior furloughs during the 2018-2019 government shutdown "built a sense of urgency to accomplish projects to 'catch up,'" the report stated.

A scorched structure and vehicle stand on a property mostly destroyed by the Hermits Peak/Calf Canyon Fire on June 2 near Las Vegas, New Mexico. (Mario Tama/Getty Images)
The prescribed burn in New Mexico was started in April and almost immediately took an unexpected turn. “Within hours of declaring the test fire a success that day, multiple spot fires were reported outside containment lines and there were not enough resources or water to rein them in,” the Washington Post reported.

As of Tuesday, the Calf Canyon/Hermits Peak Fire had burned 533 square miles, making it the largest fire so far this year in the United States. The area burned nationally this year — 5,000 square miles — is more than two and half times the national average for the past 10 years at this point in the season, according to the National Interagency Fire Center.

In addition to causing warmer temperatures, climate change significantly impacts the water cycle, both of which experts say contributed to the conditions that resulted in the New Mexico fire getting out of hand.

"Along with below normal precipitation, the seasonal snowpack was significantly compressed, as it did not start until January then abruptly melted off much earlier than average," the report stated.

The Forest Service will have to more effectively factor climate change into its plans, the report stated.

“Fires are outpacing our models and, as the final report notes, we need to better understand how megadrought and climate change are affecting our actions on the ground,” Moore concluded.
'Moment of reckoning:' Federal official warns of Colorado River water supply cuts
[title]

The Colorado River’s reservoirs have diminished to the point that significant cuts to the water supplied to the seven states that rely on it will be necessary next year, a federal official warned Tuesday.

Bureau of Reclamation Commissioner Camille Calimlim Touton told the Senate Energy and Natural Resources Committee maintaining “critical levels” at the largest reservoirs in the United States — Lake Mead and Lake Powell — will require large reductions in water deliveries.

“A warmer, drier West is what we are seeing today,” she said at a hearing. “And the challenges we are seeing today are unlike anything we have seen in our history.”
From above, a river flows through a rocky desert landscape.
The relatively arid desert Southwest is viewed at 33,000 feet on May 19 near Moab, Utah. The Colorado River, flowing from Colorado's Rocky Mountain through Utah, Arizona, Nevada and California is dependent on winter snowfall in the Rockies. (George Rose/Getty Images)

Colorado, New Mexico, Utah, Wyoming, Arizona, California, and Nevada all receive water from the Colorado River and next year will see a decrease of between 2 million and 4 million acre-feet of water due to the ongoing drought that has gripped most of the Western U.S. (An acre-foot is the amount of water needed to cover one acre of land in one-foot-deep water.) Current allotments of water from the Colorado range from 300,000 acre-feet for Nevada to 4.4 million acre-feet for California.

“What has been a slow-motion train wreck for 20 years is accelerating, and the moment of reckoning is near,” John Entsminger, general manager of the Southern Nevada Water Authority, told the Senate hearing. “We are 150 feet from 25 million Americans losing access to the Colorado River, and the rate of decline is accelerating.”

The West has been suffering through an acute drought since 2020, part of a megadrought that began in 2000. The last 20 years have been the driest two decades in the last 1,200 years. This year is so far the driest on record in California. Scientists attribute these conditions to climate change, which causes more water evaporation due to warmer temperatures.

“As a climate scientist, I’ve watched how climate change is making drought conditions increasingly worse — particularly in the western and central U.S.,” wrote Imtiaz Rangwala, research scientist in climate at the Cooperative Institute for Research in Environmental Sciences at the University of Colorado Boulder, in May. “The last two years have been more than 2 degrees Fahrenheit (1.1 Celsius) warmer than normal in these regions. Large swaths of the Southwest have been even hotter, with temperatures more than 3 F (1.7 C) higher.”

Western states have already been undertaking emergency measures to deal with the water scarcity. Seven months ago, California, Arizona and Nevada signed an agreement to take less water from Lake Mead, and six weeks ago the Department of Interior announced it is withholding some water from Lake Powell. Otherwise, DOI feared, the reservoir could drop so low that Glen Canyon Dam would not be able to generate electricity.

Last year, for the first time ever, the federal government declared a shortage on the river, which led to reductions in water deliveries to Arizona and Nevada. Some farmers in Arizona have had to leave some fields unplanted as a result.

Local governments and water utilities have been imposing restrictions on water usage. On June 1, the Metropolitan Water District of Southern California instituted limits on outdoor watering; typically it will be restricted to one or two days per week. But the water shortage persists.

“Despite those efforts and a previous deal among the states to share in the shortages, the two reservoirs stand at or near record-low levels,” the Los Angeles Times reported. “Lake Mead near Las Vegas has dropped to 28% of its full capacity, while Lake Powell on the Utah-Arizona border is now just 27% full.”

Touton told the Senate committee that her agency is negotiating with the seven states that depend on the Colorado River to develop a plan for apportioning the water supply reductions in the next two months. In all, nearly 40 million people rely on water from the river.

Sen. Martin Heinrich, D-N.M., attributed the gathering crisis to a lack of coordinated action to mitigate climate change.

“It’s frankly a direct result of the lack of action on climate that we have seen for more than 20 years,” Heinrich said.
Science
Earliest evidence of wildfire found in Wales
[title]

The oldest evidence of wildfire has been identified in South Wales.

It takes the form of some truly ancient, charred remnants trapped in some truly ancient mudstone.

And by ancient we're talking 430 million years ago, during the Silurian Period of Earth history.

Back then, only a few pioneering plants had made it on to land, so what was it that caught fire and produced the charcoal? Most likely it was a forest of giant fungi.

"The Silurian vegetation was very different to what it is today," explained palaeobotanist Ian Glasspool.

"There were no woody plants at this time; most of the vegetation was very small. However, there was one giant that dwarfed the landscape. There's a very enigmatic fossil called Prototaxites.

"It grew anything up to 8m in height, and about a meter in diameter. A sort of funky, humongous fungus; erect, very phallic structures; pillars of fungus that could weigh up to 10 metric tonnes," he told the Science In Action programme on the BBC World Service.

It's these strange organisms that went up in flames and left the blackened traces, Dr Glasspool believes.

His Welsh mudstone was drilled from deep under Rumney on the outskirts of Cardiff. These sediments were laid down when what is now the British Isles would have been in the Southern Hemisphere.

The rock records a near-shore marine setting, meaning the tiny fragments (2-3mm in length) of charcoal were being washed out to sea. That in itself is instructive because to have left their mark, it suggests the Prototaxites fires on land were sufficiently large and widespread.

Dr Glasspool has similar evidence from Winnica, in the Kielce region of Poland.

Together, the observations push the earliest evidence for wildfire on Earth back by about 10 million years.

And in doing so, this science reveals something else about Earth during the Silurian: the amount of oxygen in the atmosphere.

The concentration of O2 in the air today is about 21%, but early in Earth's history it was much less. It took photosynthetic algae in the oceans millions of years to terraform the planet.

Dr Glasspool said: "For fires to propagate, you really need three things: A source of fuel, which, surprisingly, we seem to have in sufficient amounts in the Silurian; you need a source of ignition, which is lightning strikes as the most likely source; and then you need at least 16% atmospheric oxygen.

"There are many geochemical proxy models that look at atmospheric oxygen, but there's quite a large discrepancy between many of them. So our charcoal data helps proof these models, and with enough data points, we can then get a better feel for how atmospheric oxygen was trending during this time interval."

Ian Glasspool reports the fire evidence with colleague Robert Gastaldo in the journal Geology.

Both scientists are affiliated to Colby College in Maine, US.
Nearly a quarter of Earth's seafloor now mapped
[title]

Slowly but surely the proportion of the global ocean floor that's been properly mapped is rising.

It's now up to just shy of a quarter of the total area under water - at 23.4%.

Better seafloor maps help us with navigation and conservation, among many other uses.

Some 10 million sq km (3.8 million sq miles) of new bathymetric (depth) data was added in the past year. This is an area broadly equivalent to the land surface of Europe.

The update was given at the second UN Ocean Conference, taking place this week in Lisbon, Portugal.

Much of this additional data comes not from recent mapping efforts, however, but simply as a result of governments, institutions and companies agreeing to open up their archives.

It's thought a further 10-15% is still squirreled away on servers, in part because the owners worry they might be giving away commercial or defense secrets if they release the information.

"But they really needn't worry," said Jamie McMichael-Phillips, director of Seabed 2030, the organization that is trying to corral world efforts to obtain a complete picture of Earth's ocean bottom.

"One of the messages we're trying to get across is that we don't require high-resolution data. Hi-res is nice; we can work with it. But lower resolution is perfectly acceptable.

"One depth value in an area the size of a European football pitch, 100m by 100m or thereabouts, isn't going to give away national or commercial secrets."

This knowledge is needed for a host of reasons.

Sea maps are essential for safe navigation, obviously, but also for fisheries management and conservation. Marine wildlife tends to congregate around the underwater mountains. Each seamount is a biodiversity hotspot.

In addition, the rugged seafloor influences the behavior of ocean currents and the vertical mixing of water. This is information required to improve the models that forecast future climate change - because it is the oceans that play a pivotal role in moving heat around the planet.

At the moment, our knowledge of just over three-quarters of the planet's underwater terrain comes only from low-resolution satellite measurements that have inferred the presence of tall seamounts and deep valleys from the gravitational influence these features have on the sea surface. Water piles up over the mass of a large submarine mountain and dips slightly where there is a trench.

It's super smart but an underwater mountain that's hundreds of meters tall can still fail to show up in such observations.

The UK's new polar ship, the RRS Sir David Attenborough, is equipped to map millions of sq km of ocean bottom over its career. The above image shows the ship's hull in dry dock. The yellow rectangle in the center is a cover made of a synthetic material over the 8m-long array of transmitting transducers for the deep-water multibeam echosounding system.

Seabed 2030, which is funded by Japan's Nippon Foundation, is encouraging anyone who ventures away from the land to switch on their sonar equipment and take depth soundings. And this isn't just about measurements from big ships; small ocean-going yachts fitted with data loggers can also make a contribution.

One of Seabed 2030's stars is the American adventurer Victor Vescovo. The Texan financier is using a submersible to visit the deepest places in the world's oceans, but everywhere he goes his support ship switches on its echosounder.

"We have a 'map the gap' strategy," Mr Vescovo told BBC News.

"We're not a commercial outfit so we don't have to follow the most fuel-efficient routes. When we go on an expedition we ask [Seabed 2030], 'what are your priority areas?'; and we divert a little bit to cover those areas."

The former US Navy reservist has himself contributed over 3 million sq km.

It's clear, however, that to come close to obtaining a full picture of the shape of Earth's ocean bottom, there will need to be a step change in approach and capability. Many parts of the world are so remote, few ships will visit them, let alone acquire depth data in those regions.

To map these places is going to require direct tasking of autonomous or semi-autonomous technologies.

There is a glimpse of how this will work in one line of data featured in the map at the top of this page. It was gathered by the Saildrone Surveyor on a cruise between San Francisco and Honolulu last year.

During this 28-day voyage, the robot boat mapped 22,000 sq km of seafloor.

Saildrone Surveyor is 22m in length. But truly huge autonomous vessels are coming.

The marine robotics company Ocean Infinity is currently building a fleet of 78m-long ships in Vietnam. Regulations will probably mean they have to be lean-crewed for the near future, but the goal eventually is to have them roving the ocean without anyone onboard. Their work would be overseen from satellite-linked control centers in the UK, the US and a third location somewhere in Asia.

Such ships could be sent out on long missions to map hard to reach areas at much lower cost than would be incurred by a conventional crewed vessel.

Progress to full mapping of the seafloor was discussed in a side meeting at this week's UN Ocean Conference. And while the participants recognised new technologies were essential to fulfilling the quest, Dr Lucy Woodall cautioned that the 2030 project would fail unless it engaged all communities with an interest in the data.

She cited examples of companies going into coastal areas to map the seafloor and then not sharing any of the information with the local people whose livelihoods depended on those waters.

"I would argue to those of you in the room who think technology has got to be the way - I would argue that, actually, people are the way because unless people are asking the questions, unless we have a dialogue with all the voices in the room, then we're not going to ask, and therefore we can't answer, those right questions," the chief scientist with Nekton, a UK-based oceans NGO, told the meeting.
Intact wooly mammoth baby uncovered in northwestern Canada
[title]

The preserved remains of a nearly whole 30,000-year-old baby woolly mammoth have been discovered in northwestern Canada.

The baby mammoth was found frozen in permafrost in the Klondike gold fields in the Yukon. Government officials and representatives of the Trʼondëk Hwëchʼin Traditional Territory, where the ancient animal was discovered, said it's the most complete and best-preserved woolly mammoth ever found in North America.

The mummified mammoth was uncovered on June 21 by miners who were digging through the permafrost on Eureka Creek, according to the Yukon government.

Dan Shugar, a geomorphologist and associate professor at the University of Calgary, helped extract the mummified mammoth. He tweeted Friday that the initiative was “the most exciting scientific thing I have ever been part of, bar none.”

Shugar said the stunningly preserved mammoth calf still has its trunk, hair, skin, toenails and intestines intact.

"It's amazing," Tr’ondëk Hwëch’in elder Peggy Kormendy said in a statement. "It took my breath away when they removed the tarp."

Researchers from the Yukon Geological Survey and the University of Calgary said the female baby likely died and became entombed in permafrost more than 30,000 years ago, during the last ice age. Elders of the First Nation Trʼondëk Hwëchʼin named the calf "Nun cho ga," which means "big baby animal" in the Hän language.

“As an ice age paleontologist, it has been one of my life long dreams to come face to face with a real woolly mammoth. That dream came true today,” Grant Zazula, a paleontologist with the Government of Yukon, said Friday in a statement.

It is only the second time a mammoth calf has been uncovered whole, according to the researchers. A separate, near-complete infant mammoth, dubbed "Lyuba," was discovered in 2007 in Siberia. Decades earlier, parts of a mammoth calf were found at a gold mine in Alaska in 1948.

Studying the remains of Nun cho ga could help scientists better understand the lives and behaviors of woolly mammoths, the researchers said. The mummified calf could also yield new insights into other ice age animals that once lived in the Yukon, they said, including cave lions and giant steppe bison.
Photo shows newly-discovered bacteria so large they are visible to the naked eye
[title]

Scientists discovered a new species of bacteria visible with the naked eye.

The bacteria, found in the Caribbean mangrove, is the biggest discovered to date.

It has other peculiarities, like internal membranes organizing its insides.

Scientists discovered a new type of bacteria that grow to the size of a human eyelash, thousands of times larger than most bacteria and the biggest seen to date.

The thin, vermicelli-like bacteria grow up to 1 cm (0.4 inches) in length, per a press release accompanying the work.

That's about 5,000 times bigger than most others and about 50 times bigger than any other known bacteria.

"It would be like a human encountering another human as tall as Mount Everest," said Jean-Marie Volland, the lead author of the study, in the press release.

The findings, published in Science on Thursday, challenge the limits of what a bacteria looks like.

The bacteria, Thiomargarita magnifica, were found by chance in Carribean mangroves by Olivier Gros, a marine biology professor at the Université des Antilles in Guadeloupe.

"When I saw them, I thought, 'Strange,'" he said in the press release, recalling being unable to identify the white filaments floating on the surface of a leaf.

The bacteria are so large they are technically no longer microbes, which are defined by being invisible to the eye.

They have other odd features: further analysis revealed complicated internal structures separated by membranes, which is unusual for a bacterium.

Cells in humans and other organisms have membranes that organize their insides into compartments, like the nucleus that contains the DNA, or the endoplasmic reticulum which helps make proteins.

But bacteria tend not to have them. Their DNA, for instance, usually floats loosely inside the cells, not encased in a membrane.

But scientists found Thiomargarita magnifica has membranes that encase its DNA. Volland dubbed this new structure a "pepin" after the French word for seeds found in fruits.

Ancient fossils in the 'Cradle of Humankind' are more than 1 million years older than previously thought
[title]

Scientists say early human ancestors, whose remains are in a South African cave, lived about 3.7 million years ago.

Researchers relied on "burial dating," a method that uses space particles to date early human fossils.

The fossils' updated age makes them several hundred thousand years older than the human ancestor "Lucy."

In 1936, archeologists began unearthing a trove of early human fossils in a South African cave. Now, researchers say most of those ancient bones date back 3.7 million years, which makes them more than 1 million years older than previously thought.

In a study published Monday in the Proceedings of the National Academy of Sciences, an international team of researchers turned to an innovative dating technique. They used space particles to analyze bones in the Sterkfontein Caves, part of a a major fossil site in northern South Africa known as the "Cradle of Humankind."

The Sterkfontein Caves contain more remains from Australopithecus — a family of early hominins that eventually gave rise to Homo sapiens — than anywhere else on Earth, according to Darryl Granger, a geology professor at Purdue University and lead researcher of the study. "There are hundreds of them," he told Insider.

But it's hard to accurately date the Australopithecus remains, in part because the cave has multiple layers, as well as animal fossils on the same site, which might be from different eras than the fossils next to them.

To gauge the ages of the hominid skeletal remains, Granger and his team used a technique known as "cosmogenic nuclide dating," or burial dating, which involves examining the rocks that encased the ancient bones. It works like this: When energetic particles from space, or cosmic rays, hit rocks, they produce elements like aluminum and beryllium that build up and decay at a known rate.

"We're able to take a rock that was exposed to cosmic rays, and if it falls into a cave, it's shielded from more radiation," Granger told Insider, adding, "It's called burial dating because, really, what we're doing is dating when the rock was buried."

Granger used the same method in 2015 to estimate that one set of Australopithecus remains found in the Sterkfontein Caves, nicknamed Little Foot, was about 3.4 to 3.7 million years old. The new study suggests that in addition to Little Foot, all Australopithecus remains on the site are between 3.4 and 3.7 million years old, rather than roughly 2 million years old, as scientists previously thought.

The remains' shifting age puts the species within roughly the same time frame that the famous human ancestor "Lucy" — which belonged to the species Australopithecus afarensis — roamed what's now Ethiopia, 3.2 million years ago. According to Granger, that refutes the theory that the Sterkfontein individuals descended from Australopithecus afarensis. "There must be an older common ancestor somewhere," Granger added.

Granger hopes the team's findings, and the burial dating method used, could help better chronicle human evolution. He hopes follow-up studies will tease out how the Sterkfontein remains compare to those found in different South African fossil sites, and beyond, he added.

Because of burial dating, he said, "We're able to make much better measurements than we could before on several human evolution sites around the world."
