# Supplementary material for: Harnessing the Power of LLMs: Evaluating Human-AI Text Co-Creation through the Lens of News Headline Generation
Source: arXiv:2310.10706 source file (2023-10-18)
Supplement: Supplementary file 2 [file study-1.tex]

Experts in news editing or curation needed for research study
Controlled experiment
zding@dataminr.com
July 2022

Job Posting
We are researchers studying how people write news headlines.

In this study, you will do a quick tutorial on creating news headlines and then create headlines for 22 news articles with our system. We will also ask questions related to your experience.

This study will take about 60 minutes, and must be performed in a single, scheduled session using a desktop or laptop computer. You will be paid $20.

We are looking for participants who have a writing or editing background, particularly in news editing or curation.

Your interactions with the tool will be logged, but all of the collected data will be kept anonymous. To participate in this study, you must be at least 18 years old, live in the United States, and agree voluntarily to participate.

\$20 fixed price
Entry level
Project type: one-time project
You will be asked to answer the following questions when submitting a proposal:
Tell us about your experience in news editing or curation, e.g., how much experience do you have writing news articles or similar content, what type of news curation have you done?
How often do you read news articles online? Please answer with the following options: "A few times a day", "A few times a week", "A few times a month", "A few times a year", and "Less than a few times a year or never"

Skills & Expertise
Writing, editor, communications, journalism writing

Preferred qualifications
Talent type: independent	
Job success score: at least 90\%
English level: native or bilingual
