# Supplementary material for: Harnessing the Power of LLMs: Evaluating Human-AI Text Co-Creation through the Lens of News Headline Generation
Source: arXiv:2310.10706 source file (2023-10-18)
Supplement: Supplementary file 3 [file study-2.tex]

Experts in news writing or editing needed for evaluating news headlines

zding@dataminr.com
August 2022

Job Posting

In this task, you will rank the quality of headlines for 20 news articles, 6 headlines per article. 
This task will take about 60 minutes, and must be performed using a desktop or laptop computer. You will be paid \$20.

We are looking for participants who have a writing or editing background, particularly in news editing or curation.

To participate in this task, you must be at least 18 years old, live in the United States, and agree voluntarily to participate.

—----

Project Details

\$20 fixed price
Entry level
Project type: one-time project
You will be asked to answer the following questions when submitting a proposal:
Tell us about your experience in news editing or curation, e.g., how much experience do you have writing news articles or similar content, what type of news curation have you done?
How often do you read news articles online? Please answer with the following options: "A few times a day", "A few times a week", "A few times a month", "A few times a year", and "Less than a few times a year or never"

Skills & Expertise
Writing, editor, communications, journalism writing

Preferred qualifications
Talent type: independent	
Job success score: at least 90%
English level: native or bilingual

—----

Comms

Note: track in google sheet who you’ve sent contract to, who has accepted, and who has completed the task, who has been paid, etc.

To applicants:

Thank you for your interest in our task! You will need to complete this task on 9 Aug (Tue). It should take about one hour and needs to be completed in one session. You need to have access to Google Sheets or Excel to complete this task (Google Sheets is preferred). If you are still interested to proceed, let me know and I will send the contract for your review. Once you’ve accepted, I’ll send instructions for completing the task.

[SEND CONTRACT]

After they’ve accepted contract:
Thank you for accepting the task! You’ll need to complete the task in a single session on or before 9 Aug (Tue). 

You will complete this task using the provided excel sheet. It is highly recommended to open the sheet sent to you with Google Sheets (for formatting).

To start the task, please upload the excel file (participant\_x.xlsx) I sent to you to Google Drive and open that with Google Sheets. Then, please follow the instructions on the instruction page (tab).

When you finish the task, please download the sheets from your Google Drive and send the .xlsx file back to me for verification.

If you have any questions, please feel free to contact me. Thank you!
