# Supplementary material for: Harnessing the Power of LLMs: Evaluating Human-AI Text Co-Creation through the Lens of News Headline Generation
Source: arXiv:2310.10706 source file (2023-10-18)
Supplement: Supplementary file 4 [file study-1-consent.tex]

Introduction
This task is a part of a research study conducted by the HAI team of Dataminr. The purpose of this study is to understand how to help people write headlines for news articles. If you have any questions, please contact Jason Ding (zding@dataminr.com) and Alison Renner (arenner@dataminr.com).

Procedures
During this task, you will complete a short tutorial before creating headlines for 20 news articles. Afterwards, you will answer a few survey questions about your experience. 

Expected Duration and Compensation
The task will take approximately 60 minutes and you will receive \$20 for your participation through the Upwork platform.

Participant Requirements
Participants must be at least 18 years old and live in the United States.

Voluntary Participation and Data Collection
Your participation is voluntary. If you would like to stop participating at any time, just let us know. This interface only captures your interaction with the system and the headlines created. We will not collect personal data in addition to that. 

By clicking the "next" button you certify the following:
1. You are 18 years of age or older and live in the United States.
2. You have read and understand the information above.
3. You want to participate in this research and continue with the headline creation task.
