# Supplementary material for: Harnessing the Power of LLMs: Evaluating Human-AI Text Co-Creation through the Lens of News Headline Generation
Source: arXiv:2310.10706 source file (2023-10-18)
Supplement: Supplementary file 5 [file prompt-programming.tex]

Prompt for keywords generation

Please identify five keywords and key phrases (nouns) for the following news article.
News article:
…
Five keywords and key phrases (nouns), separated with comma:

Prompt for headline generation with keywords

Please come up with three high-quality (attractive, clear, accurate and inoffensive) headlines for the following news article including keyword(s):
News article:
…
Three high-quality headlines:

Prompt for headline generation without keywords

Please come up with three high-quality (attractive, clear, accurate and inoffensive) headlines for the following news article:
News article:
…
Three high-quality headlines:
